# Supplementary material for: Origin of competing charge density waves in kagome metal ScV$_6$Sn$_6$
Source: arXiv:2403.17058 source file (2024-12-02)
Supplement: Supplementary file 1 [file SI.pdf]

# Supplemental Material for "Origin of competing charge density waves in kagome metal $ScV_6Sn_6$"

Kang Wang,[1] Siyu Chen,[1,2] Sun-Woo Kim,[1,*] and Bartomeu Monserrat[1,2,†]

[1]*Department of Materials Science and Metallurgy, University of Cambridge, 27 Charles Babbage Road, Cambridge CB3 0FS, United Kingdom*

[2]*Cavendish Laboratory, University of Cambridge, J. J. Thomson Avenue, Cambridge CB3 0HE, United Kingdom*

## CONTENTS

1. Calculation details 2

2. Convergence tests 3
 2.1. Convergence of phonon dispersions 3
 2.2. Cross-check with CASTEP 5

3. Comparison between PBE and PBEsol functionals 6
 3.1. Lattice parameters 6
 3.2. Harmonic phonon dispersions 6
 3.3. Potential energy surface along imaginary modes 7

4. Electronic temperature effects 8

5. CDW instabilities at zero temperature 9

6. Details about multi-phonon effects 10

7. Comparison with previous results 12

References 13

## 1. CALCULATION DETAILS

*Electronic structure calculations.* - We perform density functional theory (DFT) calculations using the Vienna *ab initio* simulation package VASP [1, 2] implementing the projector-augmented wave method [3]. We use PAW pseudopotentials with valence configurations: $3s^23p^63d^14s^2$ ($3d^14s^2$) for Sc atoms, $3s^23p^64s^23d^3$ ($4s^23d^3$) for V atoms, and $5s^24d^{10}5p^2$ ($5s^25p^2$) for Sn atoms for the cases with (without) semi-core states. We approximate the exchange correlation functional with the generalized-gradient approximation PBEsol [4] in the calculations reported in the main text. For comparison, we also perform calculations using the PBE [5] exchange-correlation functional. We use a kinetic energy cutoff for the plane wave basis of 500 eV and a Methfessel-Paxton smearing of 0.02 eV. We use a $\Gamma$-centered $\mathbf{k}$-point grid of size $15 \times 15 \times 8$ for the primitive cell and commensurate $\mathbf{k}$-point grids for the supercell calculations. All the structures are optimized until the forces are below 0.005 eV/Å.

We perform a cross-check of the electronic structure calculations using the CASTEP [6] package, with norm-conversing pseudopotentials generated on-the-fly (NCP19), and employing identical valence configurations as those used in VASP calculations, including semi-core states. We also use the PBEsol [4] exchange-correlation functional. We choose a kinetic energy cutoff for the plane wave basis of 1000 eV with a Gaussian smearing of 0.02 eV. We use a Monkhorst-Pack $\mathbf{k}$-point grid with an applied half step shift if the number of $\mathbf{k}$-points is even, which generates the exact same Gamma-centred $\mathbf{k}$-point grid as that used in the VASP calculations. All the structures are optimized until the forces are below 0.005 eV/Å.

*Harmonic phonon calculations.* - We perform harmonic phonon calculations using the finite displacement method in conjunction with nondiagonal supercells [7, 8]. The dynamical matrices are calculated on a Farey nonuniform $\mathbf{q}$ grid [9] of size $(3 \times 3 \times 2) \cup (3 \times 3 \times 3)$, which is commensurate with both $\mathbf{q}_2$ and $\mathbf{q}_3$. The final dynamical matrix is calculated through the force constant matrix on a target uniform $\mathbf{q}$ grid of size $3 \times 3 \times 6$.

*Anharmonic phonon calculations.* - The anharmonic phonon calculations are performed using the stochastic self-consistent harmonic approximation (SSCHA) [10–12], which is a non-perturbation method taking into account anharmonic effects at both zero and finite temperature. The free energy of the real system is variationally minimized with respect to an auxiliary harmonic system. This is done using stochastic importance sampling, in which the total energy, forces, and stresses for an ensemble of configurations of the auxiliary harmonic system are calculated using VASP. The associated electronic structure calculations are performed using a kinetic energy cutoff 300 eV, and we consider configurations commensurate with a $3 \times 3 \times 2$ supercell and a $3 \times 3 \times 3$ supercell. The number of configurations needed to converge the free energy Hessian is of the order of 1,000. A Farey nonuniform $\mathbf{q}$ grid of size $(3 \times 3 \times 2) \cup (3 \times 3 \times 3)$ is used to get commensurate phonon results at both $\mathbf{q}_2$ and $\mathbf{q}_3$. To get better prediction of the CDW transition temperature, the lattice parameters are fixed to the experimental values [13].

## 2. CONVERGENCE TESTS

### 2.1. Convergence of phonon dispersions

In this section, we investigate the convergence of phonon dispersions with respect to the **q**-point grid size. Since the two competing CDW orders with wave vectors $\mathbf{q}_2$ and $\mathbf{q}_3$ correspond to the H and K$^{'}$ points of the Brillouin zone, respectively, it is crucial to calculate the dynamical matrices directly at both H and K$^{'}$ points to obtain reliable results. We accomplish this using a non-uniform Farey grid [14] of size $(3\times3\times2)\cup(3\times3\times3)$, as it is computationally more efficient than the uniform grid of size $3\times3\times6$ that would otherwise be required.

Figure S1 shows the anharmonic phonon dispersions obtained with different **q**-point grid sizes at various temperatures. The minimum uniform grid that includes both H and K$^{'}$ points would be of size $3\times3\times6$, which leads to a computationally prohibitive supercell size. Instead, we investigate the smaller **q**-point grid of size $3\times3\times2$ (blue solid lines), which includes the H point but does not include the K$^{'}$ point; and the smaller **q**-point grid of size $3\times3\times3$ (red solid lines), which includes the K$^{'}$ point but does not include the H point. The results in Fig. S1 demonstrate that the phonon frequencies at the H and K$^{'}$ points are significantly different depending on the **q**-point grid used. At the harmonic level, the phonon frequencies at a given **q**-point are exact if that point is included in the grid used. While this is not strictly true for anharmonic phonons, we still expect that the phonon frequencies at any given point will be more accurate when the grid includes that point, as relevant phonon-phonon interaction terms are directly included in the calculation. Therefore, we used a non-uniform Farey grid [14] of size $(3\times3\times2)\cup(3\times3\times3)$, which allows us to directly access both H and K$^{'}$ points without having to use prohibitively large supercells.

Using this strategy, the results in Fig. S1 show that when using a **q**-point grid of size $3\times3\times2$ (blue solid lines), the phonon frequencies at K$^{'}$, which are obtained through Fourier interpolation, are higher than those obtained with the more accurate Farey grid (black dashed lines), leading to the absence of the $\mathbf{q}_3$ CDW order even at $T=50\,$K. Similarly, with the **q**-point grid of size $3\times3\times3$ (red solid lines), the phonon frequencies at H are interpolated, and are significantly lower than those obtained with the Farey grid (black dashed lines), resulting in them being imaginary even at $T=200\,$K. These artificial features of Fourier interpolation can only be rectified by explicitly including both H and K$^{'}$ points, as done with the Farey grid (black dashed lines), and these are the results presented in the main text.

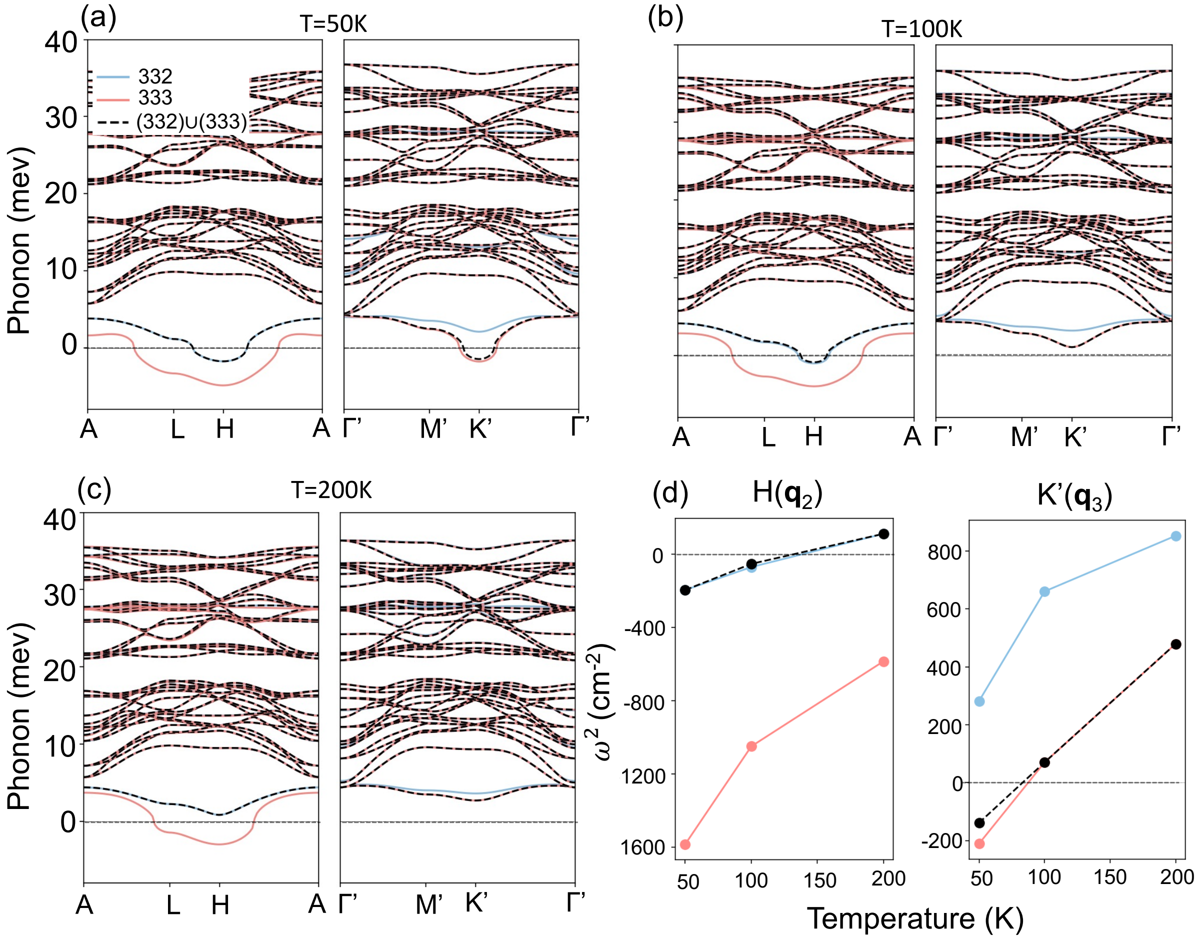


Figure S1. Calculated anharmonic phonon dispersions using **q**-point grid sizes of $3 \times 3 \times 2$, $3 \times 3 \times 3$, and $(3 \times 3 \times 2) \cup (3 \times 3 \times 3)$ at (a) 50 K (b) 100 K and (c) 200 K. (d) The square of the lowest phonon frequency ($\omega^2$) at the H ($\mathbf{q}_2$) and K$'$ ($\mathbf{q}_3$) points.

### 2.2. Cross-check with CASTEP

To cross-check the results obtained from VASP, we perform calculations using CASTEP on the two CDW structures with the same valence configurations including semi-core states. The results from both VASP and CASTEP consistently show that the $\mathbf{q}_3$ CDW order is stable over the $\mathbf{q}_2$ CDW (Table S1). Specifically, the energy difference between the two CDW structures is 0.5 meV/f.u. and 1.1 meV/f.u. using VASP and CASTEP, respectively.

Table S1. The total energy (meV/f.u.) of fully relaxed CDW structures compared to pristine structure.

| | $\mathbf{q}_2$ CDW | $\mathbf{q}_3$ CDW | $E(\mathbf{q}_2) - E(\mathbf{q}_3)$ |
|---|---|---|---|
| VASP | $-1.95$ | $-2.42$ | 0.47 |
| CASTEP | $-1.54$ | $-2.66$ | 1.12 |

## 3. COMPARISON BETWEEN PBE AND PBESOL FUNCTIONALS

### 3.1. Lattice parameters

In the main text, we present the results obtained using the PBEsol exchange-correlation functional, as it yields a better agreement with the experimentally measured out-of-plane lattice parameter, a quantity that is crucial for CDW formation. Specifically, PBEsol gives an out-of-plane lattice parameter of $c = 9.12$ Å, which is closer to the experimental value of $c = 9.16$ Å compared to the PBE value of $c = 9.25$ Å (Table S2).

Table S2. Lattice parameters of pristine $ScV_6Sn_6$ obtained using PBE and PBEsol.

| Lattice parameter | PBE | PBEsol | Expt. [13] |
|---|---|---|---|
| In-plane a (Å) | 5.46 | 5.39 | 5.47 |
| Out-of-plane c (Å) | 9.25 | 9.12 | 9.16 |

### 3.2. Harmonic phonon dispersions

Figure S2 shows the calculated phonon dispersions using PBEsol and PBE. The overall phonon dispersions look similar, including the imaginary branches. Both PBEsol and PBE show phonon instabilities at the H and K$'$ points, and the largest magnitude instability is observed at the H point.

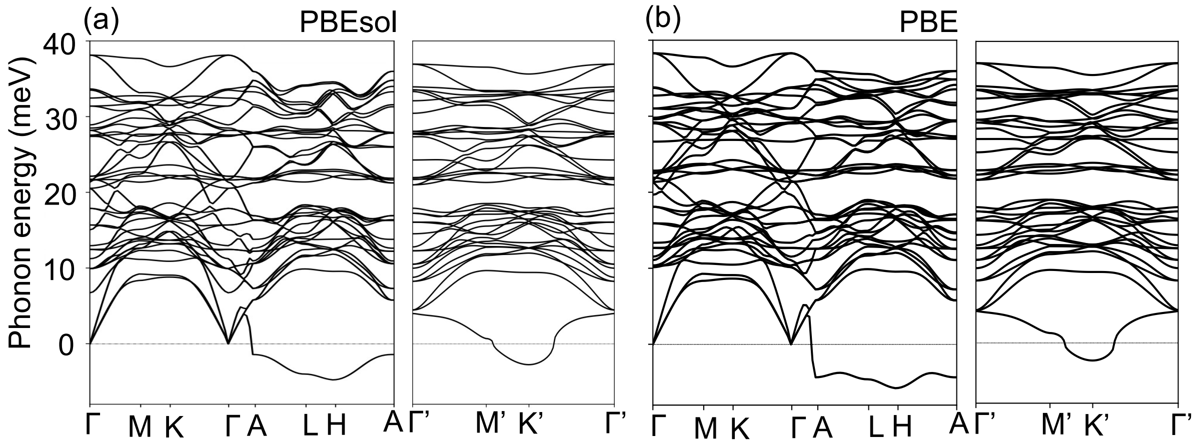


Figure S2. The harmonic phonon dispersions obtained using the (a) PBEsol and (b) PBE functionals. A Farey grid of size $(3 \times 3 \times 2) \cup (3 \times 3 \times 3)$ is used to obtain the phonon dispersions.

### 3.3. Potential energy surface along imaginary modes

In Fig. 3 of the main text, we present the total energy of the $\mathbf{q}_2$ and $\mathbf{q}_3$ CDWs by displacing the pristine structure with a single phonon mode at H and K$^{'}$ points, respectively. Here, we provide the detailed calculation results and compare the results obtained using the PBE and PBEsol functionals. Figures S3(a) and S3(b) show the potential energy surface calculated using PBEsol with and without including the semi-core states in the valence. As discussed in the main text, the inclusion of the semi-core states reduces the energy gain of both CDW orders. Similarly, the PBE results [Figs. S3(c) and S3(d)] show a decrease in the energy gain of the CDW states upon including the semi-core states. It should be noted that the larger energy gain of the two CDW orders in PBE compared to PBEsol is due to the larger out-of-plane lattice parameter predicted by PBE, providing more space for distortion of Sn1-Sc-Sn1 trimers. Overall, both PBEsol and PBE consistently predict $\mathbf{q}_2$ to be more stable distortion when a single phonon mode is considered.

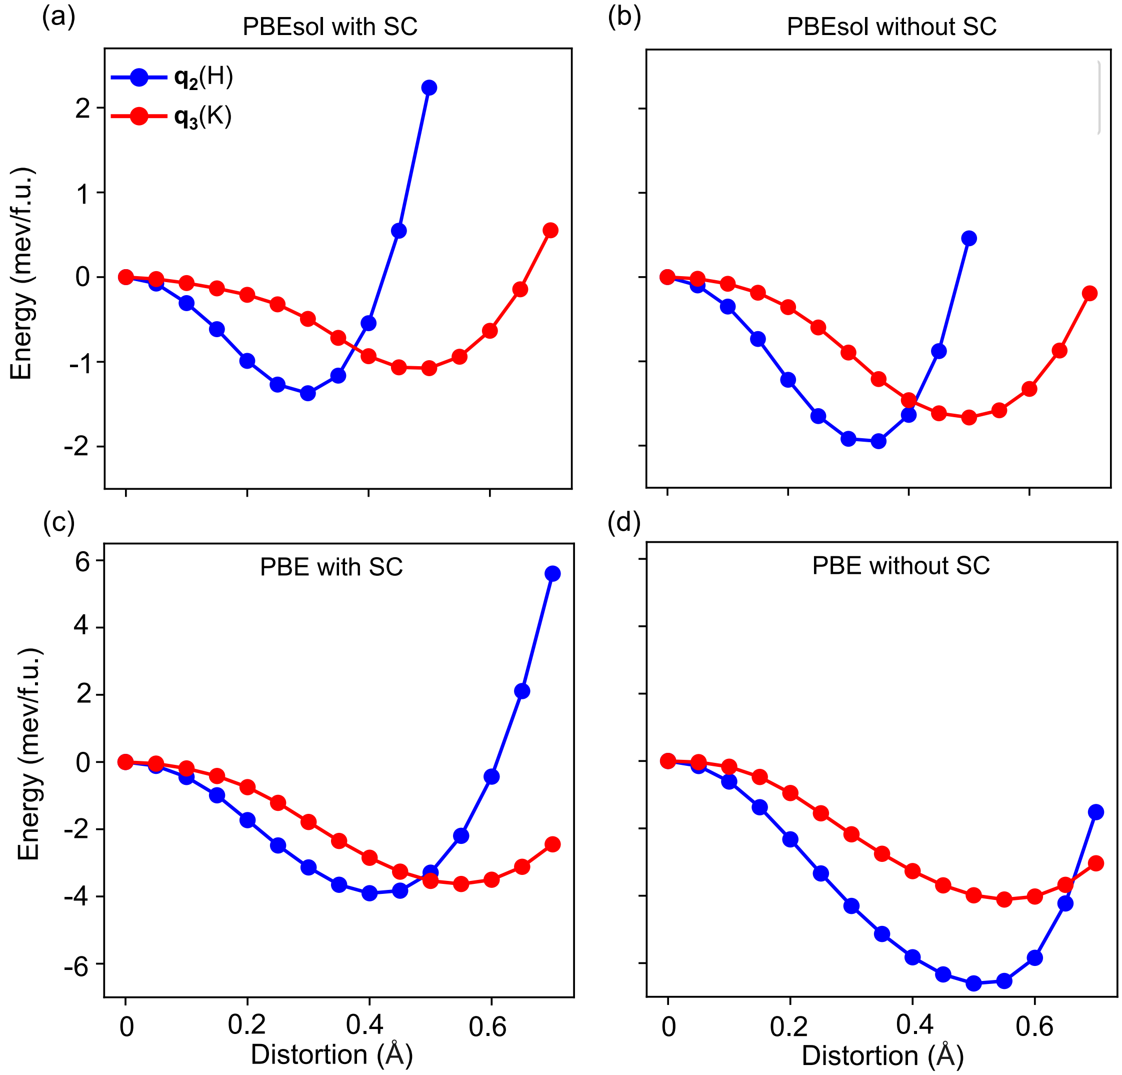


Figure S3. Calculated potential energy surface along the single phonon mode at the H ($\mathbf{q}_2$) and K$^{'}$ ($\mathbf{q}_3$) points. PBEsol results: (a) including and (b) excluding semi-core states in the valence. PBE results: (c) including and (d) excluding semi-core states in the valence.

## 4. ELECTRONIC TEMPERATURE EFFECTS

In this section, we investigate the effects of electron temperature on harmonic phonon dispersions. We calculate harmonic phonon dispersions over a range of smearing values from 0.02 eV to 0.5 eV, corresponding approximately to temperatures ranging from 300 K to 5,800 K [Fig. S4(a)]. The phonon dispersions undergo changes with increasing electronic temperature, notably in the imaginary branches. The estimated transition temperatures for the $\mathbf{q}_2$ and $\mathbf{q}_3$ CDWs are 5500 K and 2000 K, respectively [Fig. S4(b)].

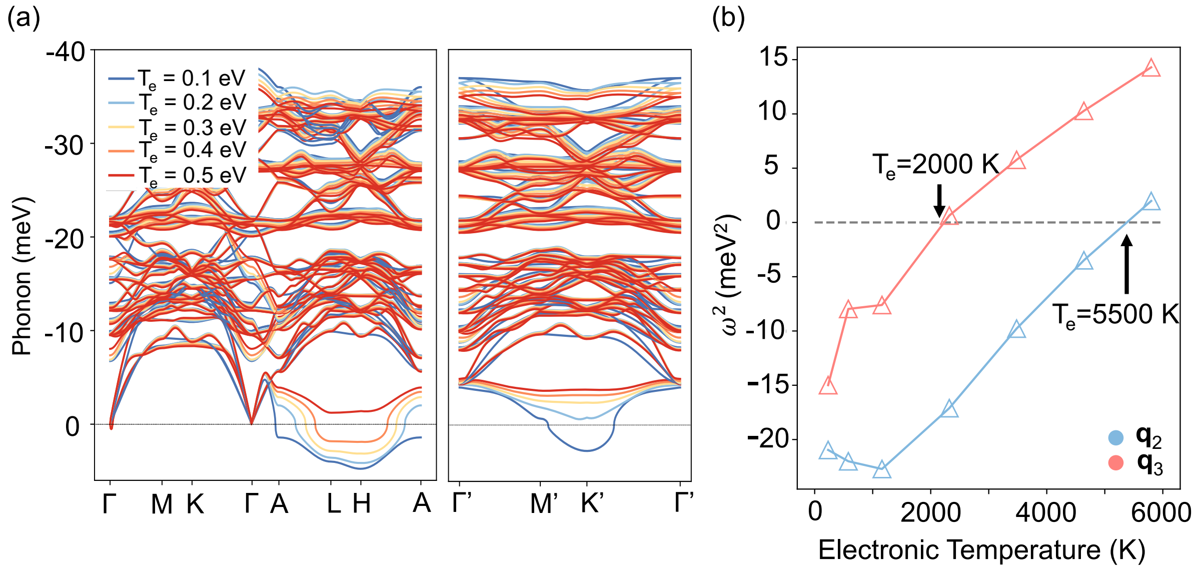


Figure S4. (a) The calculated harmonic phonon dispersion using various electronic temperature. (b) Squared phonon frequency $\omega^2$ of the lowest energy phonon modes at the H and K′ points with respect to the electronic temperature. Note that 0.1 eV is 1160.6 K.

## 5. CDW INSTABILITIES AT ZERO TEMPERATURE

As discussed in the main text, at finite temperatures, anharmonic phonon-phonon interactions lift most harmonic instabilities except those at the K′ and H points, explaining experimental observations. At zero temperature, the anharmonic zero-point energy correction already lifts the harmonic instability at the A point, while CDW instabilities persist at the K′, H, and L points [see Fig. 2(a) in the main text]. For completeness, this section delves into the energetics of these three CDW instabilities at zero temperature (Fig. S5), demonstrating that $\mathbf{q}_3$ CDW is the most stable ground state, followed by the $\mathbf{q}_2$ CDW. Our results show that the L CDW is the least stable at various levels of theory such that it cannot be observed even at very low temperatures.

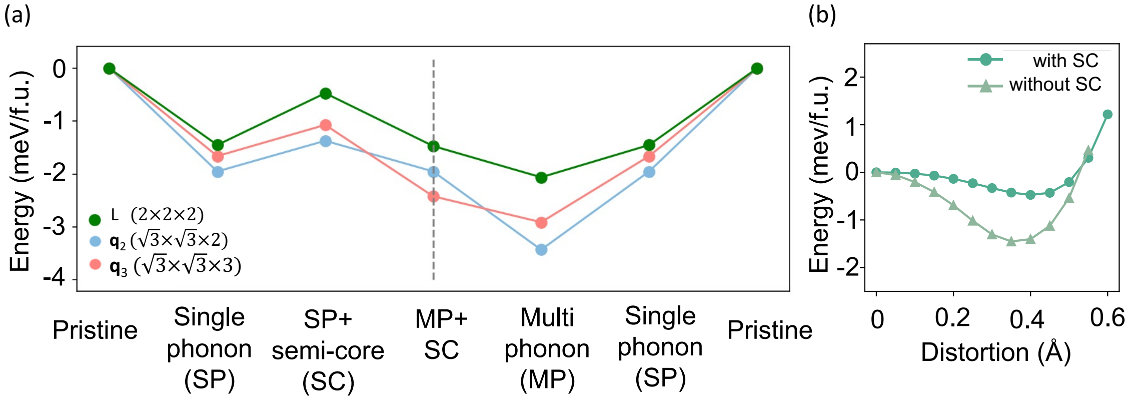


Figure S5. (a) Total energy of the $\mathbf{q}_2$,$\mathbf{q}_3$ and L CDW structures compared to the pristine structure. Single phonon (SP) and multiple phonon (MP) indicate CDW structures distorted according to the atomic displacement pattern associated with a single phonon mode or with multiple phonon modes, respectively. Semi-core (SC) refer to calculations in which $s$ and $p$ semi-core states in Sc atoms and $d$ semi-core states in Sn atoms are treated as valence states. (b) The potential energy surface of the L CDW structure.

## 6. DETAILS ABOUT MULTI-PHONON EFFECTS

In a typical potential energy surface calculation, the atoms of the high-symmetry pristine structure are distorted according to the displacement pattern provided by the eigenvector associated with the imaginary mode. For an imaginary mode, the resulting *single-mode* potential energy surface (Fig. S3) typically exhibits a “double-well” type shape, with the pristine structure corresponding to the central local maximum, surrounded by two minima that correspond to lower-energy structures. While the vast majority of potential energy surface calculations for CDW systems rely on this single-mode potential, there is no physical justification for this. The system will, in general, relax to the *overall* lowest energy point of the potential energy surface, and such a point may or may not correspond to the minima identified with the single-mode calculation. Therefore, *all* first principles calculations following an imaginary mode should be followed by a full relaxation, as we have done in our work. This subsequent relaxation will either leave the system unchanged (if the single-mode miminum is indeed the global minimum), or it will lead to a lower energy structure. Our calculations clearly reveal that in $ScV_6Sn_6$, these multi-phonon effects are critical to obtain the correct ground state (see Fig. 3 in the main text).

Having established the general principles behind relaxations starting from imaginary phonon modes, we move to discuss the case of $ScV_6Sn_6$ in detail. In $ScV_6Sn_6$, $\mathbf{q}_3$ is associated with four degenerate modes: $(\frac{1}{3},\frac{1}{3},\frac{1}{3})$, $(-\frac{1}{3},\frac{2}{3},\frac{1}{3})$, $(-\frac{1}{3},-\frac{1}{3},-\frac{1}{3})$ and $(\frac{1}{3},-\frac{2}{3},-\frac{1}{3})$. The corresponding eigenvectors are depicted in Fig. S6(a). Since they are degenerate, any linear combination of those four modes provides a valid basis for the degenerate subspace. By first distorting the structure along one of the four degenerate modes, and then relaxing it further, we allow for all harmonic degenerate modes to contribute irrespective of the arbitrary basis we started with. Using this procedure, in our calculations we confirm that first distorting the pristine structure along any of the four degenerate modes, and then further relaxing the structure ends up in the same CDW structure, which in all cases has a lower energy compared to the four single-mode structures. The structural difference between the final CDW structure and the initial high-symmetry pristine structure is shown in Fig. S6(b). Our final CDW structure is consistent with the experimentally reported CDW pattern.

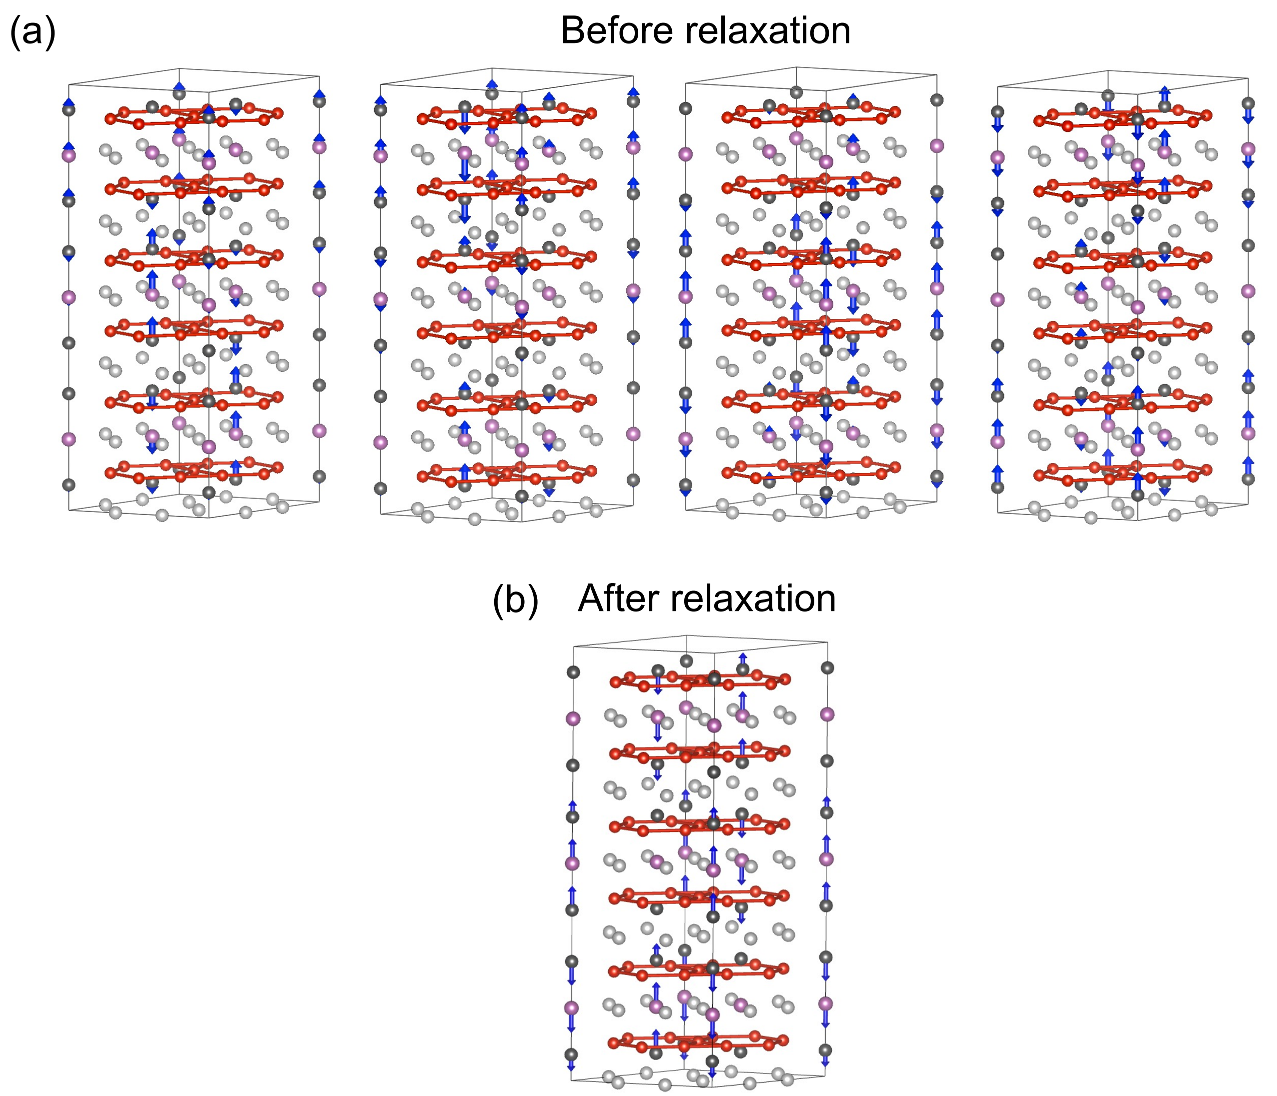


Figure S6. (a) The pristine structure with the arrows indicating the degenerate eigenmodes of $\mathbf{q}_3$ (b) The pristine structure with the arrows indicating the structural difference between the pristine and the CDW structure after relaxation.

## 7. COMPARISON WITH PREVIOUS RESULTS

In this section, we calculate the energetics of the two competing CDW states as a function of the lattice parameter (Fig. S7). This allows us to rationalize the previous reports and explain why they obtained a $\mathbf{q}_2$ CDW ground state rather than the experimentally observed $\mathbf{q}_3$ CDW ground state. The previous DFT calculations [15–19] were performed using the PBE functional, yielding an optimized out-of-plane lattice parameter of $c = 9.25$ Å, which is significantly larger than the experimental out-of-plane lattice parameter of $c = 9.16$ Å [13]. At the PBE-optimized lattice parameters, the $\mathbf{q}_2$ CDW is indeed calculated to be more stable than the $\mathbf{q}_3$ CDW (triangle in Fig. S7). However, using the experimentally reported lattice parameters shows the $\mathbf{q}_3$ CDW is ground state (star in Fig. S7). These results confirm the important role that the out-of-plane lattice parameter plays in determining the relative stability of the two CDW orders. The results also explain why previous DFT calculations failed to predict the $\mathbf{q}_3$ CDW ground state even if some of them considered the inclusion of the semi-core states in the valence states.

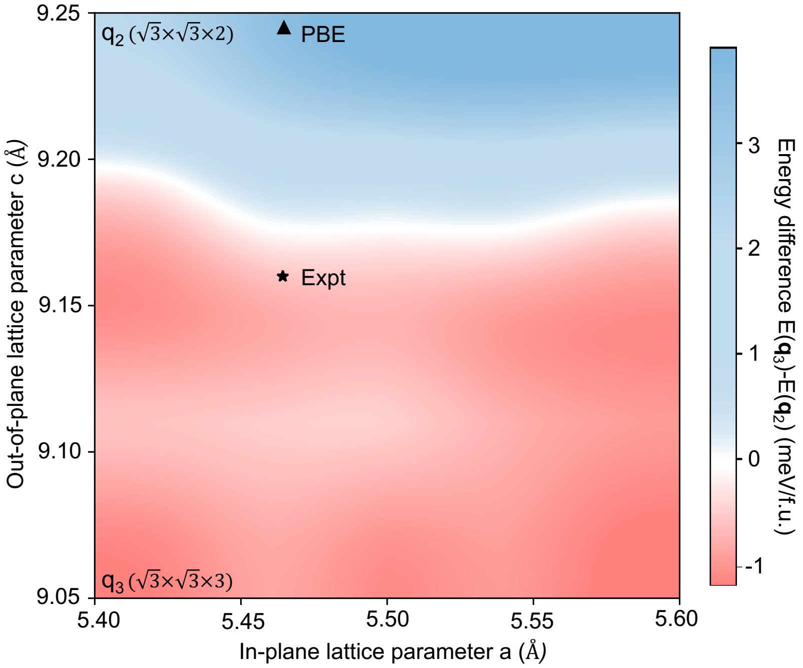


Figure S7. Calculated phase diagram as a function of lattice parameters using the PBE functional. The color bar represents the energy difference between the $\mathbf{q}_2$ and $\mathbf{q}_3$ CDW structures. The triangle corresponds to the lattice parameters obtained using the PBE functional, while the star represents the lattice parameters reported experimentally [13].

* swk38@cam.ac.uk
† bm418@cam.ac.uk

[1] G. Kresse and J. Furthmüller, Comp. Mater. Sci. **6**, 15 (1996).
[2] G. Kresse and J. Furthmüller, Phys. Rev. B **54**, 11169 (1996).
[3] P. E. Blöchl, Phys. Rev. B **50**, 17953 (1994).
[4] J. P. Perdew, A. Ruzsinszky, G. I. Csonka, O. A. Vydrov, G. E. Scuseria, L. A. Constantin, X. Zhou, and K. Burke, Phys. Rev. Lett. **100**, 136406 (2008).
[5] J. P. Perdew, K. Burke, and M. Ernzerhof, Phys. Rev. Lett. **77**, 3865 (1996).
[6] S. J. Clark, M. D. Segall, C. J. Pickard, P. J. Hasnip, M. I. J. Probert, K. Refson, and M. C. Payne, Z. Kristallogr. **220**, 567 (2005).
[7] J. H. Lloyd-Williams and B. Monserrat, Phys. Rev. B **92**, 184301 (2015).
[8] B. Monserrat, J. Phys. Condens. Matter **30**, 083001 (2018).
[9] S. Chen, P. T. Salzbrenner, and B. Monserrat, Phys. Rev. B **106**, 155102 (2022).
[10] I. Errea, M. Calandra, and F. Mauri, Phys. Rev. B **89**, 064302 (2014).
[11] R. Bianco, I. Errea, L. Paulatto, M. Calandra, and F. Mauri, Phys. Rev. B **96**, 014111 (2017).
[12] L. Monacelli, R. Bianco, M. Cherubini, M. Calandra, I. Errea, and F. Mauri, J. Phys.: Condens. Matter. **33**, 363001 (2021).
[13] H. W. S. Arachchige, W. R. Meier, M. Marshall, T. Matsuoka, R. Xue, M. A. McGuire, R. P. Hermann, H. Cao, and D. Mandrus, Phys. Rev. Lett. **129**, 216402 (2022).
[14] S. Chen, P. T. Salzbrenner, and B. Monserrat, Phys. Rev. B **106**, 155102 (2022).
[15] H. Tan and B. Yan, Phys. Rev. Lett. **130**, 266402 (2023).
[16] S. Liu, C. Wang, S. Yao, Y. Jia, Z. Zhang, and J.-H. Cho, arXiv 10.48550/arXiv.2308.13796 (2023).
[17] A. Subedi, arXiv 10.48550/arXiv.2308.11553 (2023).
[18] H. Hu, Y. Jiang, D. Călugăru, X. Feng, D. Subires, M. G. Vergniory, C. Felser, S. Blanco-Canosa, and B. A. Bernevig, arXiv 10.48550/arXiv.2305.15469 (2023).
[19] S. Cao, C. Xu, H. Fukui, T. Manjo, Y. Dong, M. Shi, Y. Liu, C. Cao, and Y. Song, Nat. Commun. **14**, 7671 (2023).
